# Supplementary material for: Capturing Evolution Genes for Time Series Data
Source: arXiv:1905.05004 source file (2022-07-12)
Supplement: Supplementary file 1 [file appendix.tex]

%!TEX root = chronos.tex

\section{Supplementary Materials}
\label{sec:appendix}
\subsection{Pseudo Code}
In order to improve the reproducibility of our method, we illustrate the structure and procedure of the \methodraw, and present the complete pseudo code of \methodname~ on the event prediction of time series. 
Given the time series $\mathcal{X} \in \mathbb{R}^{N \times T \times S}$, feature events $\mathcal{Y}$,  \method first learns different genes on all segments $\mathcal{X}_n$. Then, it combines the recognition $\mathcal{A}_n$ on the $\mathcal{X}$ and fuse the patterns from genes by the recursive structure. The application layer turns into the predicted events and back propagates the cross-entropy loss to train the whole networks. \alref{alg:1} presents more details.
\begin{figure}[htb]
	\vspace{-1em}
	\centering
	\begin{minipage}{.95\linewidth}
		\begin{algorithm}[H]

			\caption{\textbf{~The procedure of event prediction on the \methodname}}
			\label{alg:1}
			\begin{algorithmic}[1]
				\Require time series $\mathcal{X} \in \mathbb{R}^{N \times T \times S}$, event labels $\mathcal{Y}$, number of gene $K$
				\Ensure predicted label $\mathcal{Y}'$
				
				\Procedure{OuterGenes}{$\mathcal{X}$} \Comment{Capture the evolution genes}
				\State $\mathcal{A}^{(0)} \in \mathbb{R}^{N \times K} \gets$ compute the initial recognition as \equationref{eq:initial}
				\While{the error rate $\frac{|\mathcal{A} \ominus \mathcal{A}'|}{|\mathcal{A}|}$ has not converged}
				\State $\mathcal{A} = \mathcal{A}'$
				\While{$\theta_{\mathbf{D}}$, $\theta_{\mathbf{G}}$ and $\theta_{\mathbf{C}}$ have not converged}
				\State Sample $\{\mathcal{X}_n^{(m)}, \mathcal{A}_n^{(m)}\}_{m=1}^M \sim p_r$ a batch from real segments and gene recognition $\mathcal{A}_n$
				\State $\theta_{\mathbf{C}} \leftarrow \nabla_\theta[\frac{1}{M}\sum_{m=1}^{M} \mathcal{L}_{\mathbf{C}}^{(m)}]$ 
				\State $\mathcal{A}' = \arg \max \mathbf{C}(\mathcal{X})$ 
				\For{$k \gets \arg \max(\mathcal{A}')$}
				\State  $\theta_{\mathbf{D}} \leftarrow \nabla_\theta[\frac{1}{M}\sum_{m=1}^{M} \mathcal{L}_D^{(m)}]$ \Comment {Update discriminator's parameters according to \equationref{eq:discriminator}}
				\State $\theta_{\mathbf{\mathbf{E}}}, ~ \theta_{\mathbf{\mathbf{G}_i}} \leftarrow \nabla_\theta[\frac{1}{M}\sum_{m=1}^{M} (\mathcal{L}_{KL}^{(m)} + \mathcal{L}_{GD}^{(m)})]$ \Comment{Update genes' parameters according to \equationref{eq:likelihoods} and \equationref{eq:generator} }
				\EndFor
				\EndWhile
				\EndWhile
				\State $\mathbf{h} \gets \mathbf{E}(\mathcal{X}, \mathcal{A})$
				\State \Call{GenePredict}{$\mathcal{X}, \mathcal{A}, \mathbf{h}$}
				\EndProcedure
				\\
				
				\Procedure{GenePredict}{$\mathcal{X}, \mathcal{A}, \mathbf{h}$}
				\While{the parameters of \method have not converged}
				\State Sample $\{\mathcal{X}^{(\eta)}, \mathcal{A}^{(\eta)}, \mathbf{h}^{(\eta)}\} $ a batch from $(\mathcal{X}, \mathcal{A}, \mathbf{h})$
				\For{each time window $n \in N$} \Comment{Recurrence in time}
				\State $\mathcal{Q}_n\gets [\mathcal{Q}_{n-1}, \mathcal{X}_n, \mathcal{A}_n, \mathbf{h}_n]$ \Comment{Feature fusion} 
				\EndFor
				\State $\Psi(\mathcal{Q}_N) \gets$ Abstract the last output for prediction task \Comment{``end-to-end'' mechanism}
				\State $\theta_{app} \gets \nabla_\theta \left[\frac{1}{\eta}\sum_{n=1}^{\eta} (\mathcal{L})\right]$ \Comment{Back propagate the loss and train the whole \methodraw}
				\State $\theta_{\mathbf{E}}, \theta_{\mathbf{G}} \gets \alpha \times \nabla_\theta \left[\frac{1}{\eta}\sum_{n=1}^{\eta} (\mathcal{L})\right]$ \Comment{Lower learning rate for the adjustment}
				
				\EndWhile
				\EndProcedure
				
			\end{algorithmic}  
		\end{algorithm}
	\end{minipage}
	\vspace{-1em}
\end{figure}

\subsection{Implementation Details}
\vpara{Classification.} 
Time series from different sources have different formats, whose detailed statistics are as following:
\begin{table}[h]
	\centering
	\small 
	
	\addtolength{\tabcolsep}{-0pt}
	\caption{Dataset statistics}
	\begin{tabular}{l|cccc}
		\hline
		Dataset  & \#samples & \#time windows &  \#time points & \#variable \\ 
		\hline
		Synthetic & 50,000 & 10 & 20 & 3  \\
		Earthquakes & 461 & 21 & 24 & 1 \\
		\kaggletraffic & 142753 & 12 & 30 & 1 \\
		\timedataset & 3,833,213 & 12 & 4 & 2 \\
		\flowdataset & 241,045 & 15 & 24 & 2 \\
		\trafficdataset & 16,792 & 3 & 30 & 12 \\
		\hline 
	\end{tabular}
	\normalsize
	\label{tb:exp:dataset}
\end{table}

For the different datasets, if there are clear train/test split, such as UCR datasets, we use them to make experiment. Otherwise, we split the train/test set by 0.8 at the time line, such that preceding windows’ series are used for training and the following ones are used for testing. We split 10\% samples from train set as validation, which controls the procedure of training and avoids the overfitting. 

For all experiments, we set the hidden dimensions as 32 and 128 for hidden vector $\mathbf{h}$ and recurrent vector $\mathcal{Q}$ respectively. We train on an 1-GPU machine and set 2000 for a batch. Specially, for the small-size datasets from UCR, we set 50 for a batch.
The iterations of gene recognition are 5 and the training epochs of genes are 30, which have the best performance as \figref{fig:para} shows. We use the learning rate of 0.01 and 0.001 to train classifier and genes initially.
Then, we train gene application for 100 iterations in total, starting with a learning rate of 0.01 and reducing it by a factor of 10 at every 20 iterations, and use learning rate of 0.0001 to adjust the gene recognition and gene generation.
The larger the volume of the data, the more the number of batches, and the fewer training epoch required for convergence. For example, \timeshort~dataset is only trained for 30 epochs and can achieve convergence, which we train 100 epochs on Earthquakes dataset.
